# Supplementary material for: Sparse Bayesian Inference of Multivariable ARX Networks
Source: arXiv:1605.09543 source file (2019-01-03)
Supplement: Supplementary file 1 [file CDC_final_SI.pdf]

# On Identification of Dynamical Structure Functions: A Sparse Bayesian Learning Approach

J. Jin, W. Pan, D. L.T. Pham, Y. Yuan<sup>†</sup>, C. J. Tomlin, A. Webb, J. Gonçalves

**Abstract**—This paper considers the identification of linear time-invariant networks, also known as dynamic structure functions. Assuming identifiability of the network addressed in previous work, this paper presents an identification method that infers both the Boolean structure of the network and the transfer functions between nodes. The identification is performed directly from data and without any prior knowledge of the system, including its order. The method is to formulate the identification as a linear regression problem together with penalties for complexity, both in terms of element (order of nonzero connections) and group sparsity (network topology). We then propose a novel scheme that combines sparse Bayesian and sparse group Bayesian to efficiently solve the problem. The method and the developed toolbox can now be used to infer networks from a wide range of fields, including systems biology applications such as signalling and genetic regulatory networks.

## I. INTRODUCTION

Network identification of biochemical reaction networks has been a central topic in systems biology. Its first objective consists of reconstructing Boolean structures or network topologies. The next step aims at identifying the internal dynamics between nonzero nodes [2], [3], [13]–[15]. Such dynamics can be complex, involving nonlinear ODEs that typically obey biochemical kinetic laws such as mass action functions, Michaelis-Menten functions and Hill functions [10]. Building such networks demands prior knowledge of the exact type of nonlinearities and full state measurements, which is often unrealistic [16]. Sometimes, however, the dynamics may be reasonably approximated by linear systems. A major advantage is that linear systems no longer require full state measurements. For a network, linear dynamics between nodes can be described by dynamical structure functions (DSF), which focuses on the casual relationships among measured states (nodes), while suppressing the structure of hidden (not-measured) states [11], [12]. This paper infers DSF from time-series data of the measured nodes.

Since data usually contains noise, modelling DSF can lead to model over-fitting. In particular, a simple linear

regression is likely to return a fully connected network with high dimensional subsystems between nodes. As in classical system identification, to avoid these situations we need to penalise for complexity, both in terms of network topology and individual system dimension. Methods to recover such DSF can be classified into two categories [18]. Type I method, called sparse group lasso, solves the problem by introducing a penalty that blends lasso and group lasso [20]. Type II uses instead the Bayesian perspective called sparse Bayesian learning (SBL). While element SBL [16], [18], [22], [25] and group SBL [2], [17], [19], [21] have already been developed to find the sparse or group-sparse solution of a linear regression problem, no similar approach is available to search for a solution possessing both features at the same time. This paper proposes a scheme to combine SBL and group SBL, to generate sparse networks with internal dynamics described by strictly proper transfer functions with the lowest order possible.

The paper is organised as follows. Section II introduces the DSF and discusses its identifiability. Section III formulates the network reconstruction problem and casts it as a linear regression problem. Section IV solves the problem of network identification using a combination of SBL and group SBL. Section V extends the formulation to a more general case and demonstrates the underlying mechanisms of our method. Section VI applies the method to a randomly generated network and shows how its topology and internal dynamics can be reconstructed almost exactly. Finally, Section VII concludes and discusses further development in this field.

*Notation:* The notation in this paper is standard.  $I$  denotes the identity matrix. For  $L \in \mathbb{R}^{n \times n}$ ,  $\text{diag}\{L\}$  denotes a vector with its elements to be the diagonal elements of matrix  $L$ .  $\text{tr}\{L\}$  denotes the trace of matrix  $L$ . A matrix  $L \succeq 0$  means  $L$  is positive semi-definite. A vector  $v \geq 0$  means each element of the vector is non-negative. A vector  $y(t_1 : t_2)$  denotes a row vector  $[y(t_1) \ y(t_1 + 1) \ \cdots \ y(t_2)]$ .

## II. MODEL FORMULATION

In a particular experiment, the choice of measurements and what non-measured nodes (hidden nodes) represent influence the network. This paper assumes the states of the system have been defined so that the network formed by their interactions is well defined. In biology, for example, the states typically are concentrations (or number) of molecules. Consider a linear model given by its state space dynamics (without noise):

$$\begin{aligned} x(t+1) &= Ax(t) + Bu(t) \\ y(t) &= Cx(t) \end{aligned} \quad (1)$$

Junyang Jin and Alex Webb are with Circadian Signal Transduction Group, Department of Plant Sciences, University of Cambridge. Wei Pan is with Cardwell Investment Tech and Imperial College London. Duong L.T. Pham is with the Luxembourg Centre for Systems Biomedicine. Ye Yuan and Claire J. Tomlin are with the Department of Electrical Engineering and Computer Sciences, UC Berkeley. Jorge Gonçalves is with the Department of Engineering, University of Cambridge and the Luxembourg Centre for Systems Biomedicine. <sup>†</sup>For correspondence, yy311@berkeley.edu

Due to page limit, the supporting information of this paper is available from <http://hybrid.eecs.berkeley.edu/~yeyuan/cdc16.pdf>

where  $x \in \mathbb{R}^n$  are the states of the system,  $u \in \mathbb{R}^m$  the inputs, and  $y \in \mathbb{R}^p$  the measurements. To simplify notation, the paper assumes that the first  $p$  states correspond to the measurements (outputs), followed by hidden states, so that  $C$  can be written as  $C = [I \ 0]$ . For example, in systems biology there are typically a relatively small number of measurements and a large number of non-measured (hidden) species. Hence, the system can be partitioned as

$$\begin{bmatrix} y(t+1) \\ h(t+1) \end{bmatrix} = \begin{bmatrix} A_{11} & A_{12} \\ A_{21} & A_{22} \end{bmatrix} \begin{bmatrix} y(t) \\ h(t) \end{bmatrix} + \begin{bmatrix} B_1 \\ B_2 \end{bmatrix} u(t) \quad (2)$$

where  $h \in \mathbb{R}^{n-p}$  are the hidden states. To represent the system only at the measurements (nodes) level while encoding the hidden nodes via transfer functions between nodes, we use the notion of dynamical structure functions (DSF) [1], [11], [12]. From equation (10), DSF can be written as:

$$Y = QY + PU \quad (3)$$

where

$$\begin{aligned} Q &= (zI - D)^{-1}(W - D) \\ P &= (zI - D)^{-1}V \end{aligned} \quad (4)$$

and

$$\begin{aligned} W &= A_{11} + A_{12}(zI - A_{22})^{-1}A_{21} \\ V &= A_{12}(zI - A_{22})^{-1}B_2 + B_1 \\ D &= \text{diag}(W_{11}, W_{22} \dots W_{pp}) \end{aligned} \quad (5)$$

Here,  $Q$  is a matrix of transfer functions showing the connectivity of each node to other nodes. In addition, its diagonal elements are zero, since we are interested in network connectivity, not self loops. Similarly,  $P$  is a matrix of transfer functions relating the inputs to the nodes. Note that each element of  $Q$  and  $P$  is strictly proper indicating the causality of the network. The boolean structure of the network is reflected by the nonzero elements in  $Q$  and  $P$ , whereas the dynamics of the network are given by the transfer functions of their elements.

Given time-series data of nodes, the dynamical structure function is not necessarily identifiable unless partial structure information is available [1], [11], [12]:

*Theorem 1:* [11]. (Reconstruction with partial structure): Given a  $p \times m$  transfer function  $G$ , the dynamical structure function can be reconstructed from partial structure information if and only if  $p - 1$  elements in each column of  $\begin{bmatrix} Q & P \end{bmatrix}'$  are known that uniquely specify the component of (Q,P) in the null space of  $\begin{bmatrix} G' & I \end{bmatrix}$ .

This paper assumes the network is identifiable. In particular, a sufficient condition for identifiability is that  $P$  is diagonal, i.e., there are  $p$  experiments with only one input set to be non-zero for each experiment.

### III. RECONSTRUCTION PROBLEM FORMULATION

#### A. Problem Formulation

We add the process and measurement noise into the DSF model as:

$$Y = QY + PU + HE \quad (6)$$

where each element in  $E$  is i.i.d white Gaussian noise and they are independent.

$$\begin{aligned} Y &= \begin{bmatrix} y_1(t) \\ \vdots \\ y_p(t) \end{bmatrix}, \quad U = \begin{bmatrix} u_1(t) \\ \vdots \\ u_m(t) \end{bmatrix}, \quad E = \begin{bmatrix} e_1(t) \\ \vdots \\ e_p(t) \end{bmatrix} \\ Q &= [Q_{ij}(z^{-1})], \quad Q_{ii} = 0, \\ P &= [P_{ij}(z^{-1})], \quad H = \text{diag}(H_{ii}(z^{-1})). \end{aligned} \quad (7)$$

We regard each row of the function as an ARMAX process:

$$\begin{aligned} y_i(t) &= Q_{i1}y_1(t) + \dots + Q_{ip}y_p(t) + \dots + P_{im}u_m(t) + H_{ii}E_i(t) \\ &= \frac{D_{i1}^y(z^{-1})}{N_i(z^{-1})}y_1(t) + \dots + \frac{D_{im}^u(z^{-1})}{N_i(z^{-1})}u_m(t) + \underbrace{\frac{D_{ii}^e(z^{-1})}{N_i(z^{-1})}e_i(t)}_{\text{MA process}} \end{aligned} \quad (8)$$

so that

$$\begin{aligned} N_i(z^{-1})y_i(t) &= D_{i1}^y(z^{-1})y_1(t) + \dots + D_{im}^u(z^{-1})u_m(t) + \underbrace{D_{ii}^e(z^{-1})e_i}_{\text{MA process}} \\ y_i(t) &= D_{i1}^y(z^{-1})y_1(t) + \dots + [1 - N_i(z^{-1})]y_i(t) \\ &\quad + D_{im}^u(z^{-1})u_m(t) + D_{ii}^e(z^{-1})e_i. \end{aligned} \quad (9)$$

where

$$\begin{aligned} N_i(z^{-1}) &= \alpha_{i1}z^{-k} + \alpha_{i2}z^{-k+1} + \dots + \alpha_{ik}z^{-1} + 1 \\ D_{ij}^y(z^{-1}) &= \lambda_{ij1}^y z^{-k} + \dots + \lambda_{ij(k-1)}^y z^{-2} + \lambda_{ijk}^y z^{-1} \\ D_{ij}^u(z^{-1}) &= \lambda_{ij1}^u z^{-k} + \dots + \lambda_{ij(k-1)}^u z^{-2} + \lambda_{ijk}^u z^{-1} \\ D_{ii}^e(z^{-1}) &= \lambda_{ii1}^e z^{-k} + \dots + \lambda_{ii(k-1)}^e z^{-1} + \lambda_{iik}^e. \end{aligned} \quad (10)$$

*Remark 1:* All the terms which are known to guarantee identifiability can be moved to the left hand side of eq. (9). The expressions in the rest of the paper are changed accordingly.

Assume that  $m$  experiments are conducted with  $M$  time-series data points sampled for each node and input using Theorem 1. For the  $i$ th node, defining

$$\begin{aligned} Y_i^c &= \begin{bmatrix} y_i^c(M) \\ \vdots \\ y_i^c(k+1) \end{bmatrix} \\ A_i^c &= \left[ \begin{array}{c|c} y_1^c(M-k:M-1) & \dots & -y_i^c(M-k:M-1) \\ \vdots & \dots & \vdots \\ y_1^c(1:k) & \dots & -y_i^c(1:k) \end{array} \right] \\ w_i^j &= \begin{cases} \begin{bmatrix} \lambda_{ij1}^y & \dots & \lambda_{ijk}^y \end{bmatrix}^T & \text{if } j \leq p-1 \\ \begin{bmatrix} \lambda_{ij1}^u & \dots & \lambda_{ijk}^u \end{bmatrix}^T & \text{if } p \leq j \leq m+p-1 \\ \begin{bmatrix} \alpha_{i1} & \dots & \alpha_{ik} \end{bmatrix}^T & \text{if } j = p+m \end{cases} \\ \varepsilon_i^c(t) &= D_{ii}^e(z^{-1})e_i^c(t), \quad \Xi_i^c = \begin{bmatrix} \varepsilon_i^c(M) & \dots & \varepsilon_i^c(k+1) \end{bmatrix}^T \end{aligned} \quad (11)$$

$$Y_i = \begin{bmatrix} Y_i^1 \\ \vdots \\ Y_i^m \end{bmatrix}, w_i = \begin{bmatrix} w_i^1 \\ \vdots \\ w_i^{p+m} \end{bmatrix} \quad (12)$$

$$A_i = \begin{bmatrix} A_i^1 \\ \vdots \\ A_i^m \end{bmatrix}, \Xi_i = \begin{bmatrix} \Xi_i^1 \\ \vdots \\ \Xi_i^m \end{bmatrix},$$

eq. (9) can be written as a linear regression model:

$$Y_i = A_i w_i + \Xi_i \quad (13)$$

To reconstruct the whole network, we need to solve  $p$  independent linear regression problems in the same form due to  $p$  nodes. For simplicity, we use a unified expression for all the nodes:

$$y = Aw + \Xi \quad (14)$$

Now, we aim to solve this linear regression problem given measured data recorded in  $Y$  and  $A$ . Note that if the real network topology is sparse and the system order  $k$  is set to be much bigger than the true one (since we don't know the true system order, instead, we set an upper bound for it), the weighting vector  $w$  is both group-sparse (network is sparse) and element-sparse in each group. Therefore, we decide to solve the above optimization (14) utilising these prior knowledge using sparse Bayesian learning.

#### IV. RECONSTRUCTION VIA GE SPARSE BAYESIAN LEARNING

##### A. Sparsity inducing priors

From a Bayesian perspective, all the unknown variables in the linear regression model (14) are treated as stochastic random variables and assigned with a probability density function (PDF) individually. According to eq. (12), each block in the noise vector  $\Xi$  is a random variable following a Multivariate Gaussian distribution. Since these blocks present noise from different experiments, they are independent Gaussian. For eq. (9), as the noise in each experiment is generated by a Moving-Average (MA) process, the covariance matrix for each block possesses a symmetric Toeplitz structure. As a result, the vector  $\Xi \sim \mathcal{N}(0, \Pi)$  itself is Multivariate Gaussian whose covariance matrix has a block diagonal structure with each block to be a symmetric Toeplitz matrix. In this case, the likelihood of  $Y$  given the weighting vector  $w$  is  $p(Y|w) = \mathcal{N}(Y|Aw, \Pi)$ . Full Bayesian treatment also requires to introduce a prior distribution for  $w$ . We define a distribution  $p(w)$  in general form as:  $p(w) \propto \exp \left[ -\frac{1}{2} \sum_j g(w_j) \right]$ . If  $w$  has certain sparse properties, a prior inducing sparsity like Generalized Gaussian, Student's t and Logistic is assigned to  $p(w)$ . The function  $g(\cdot)$  of such priors is usually a concave, non-decreasing function of  $|w_j|$  [18].

Estimating  $w$  using maximum a posteriori (MAP) is intractable in this case because the posterior distribution  $p(w|y)$  is non-Gaussian and not analytical. To simplify the problem, sparse Bayesian learning approximates  $p(w|y)$  with a Gaussian distribution so that the solution is just  $E(w|y)$  and can be calculated easily. To do that, first note that

virtually all sparse priors namely super Gaussian can be presented in a variational form which yields a lower bound for the sparse prior  $p(w)$ . There are two types of variational representations; while we apply the convex type which is more general than the integral one [25].

To induce element sparsity to  $w$ , we introduce a prior  $p(w)$  as [16], [18]:

$$p(w_{ij}) = \max_{\beta_{ij} \geq 0} \mathcal{N}(w_{ij}|0, \beta_{ij}) \varphi(\beta_{ij}),$$

$$p(w_i) = \prod_{j=1}^k p(w_{ij}) = \max_{\beta_i \geq 0} \mathcal{N}(w_i|0, B_i) \varphi(\beta_i), \quad (15)$$

$$p(w) = \prod_{i=1}^{p+m} p(w_i) = \max_{\beta \geq 0} \mathcal{N}(w|0, B) \varphi(\beta).$$

where

$$w = \begin{bmatrix} w_1 \\ \vdots \\ w_{p+m} \end{bmatrix}, w_i = \begin{bmatrix} w_{i1} \\ \vdots \\ w_{ik} \end{bmatrix}$$

$$\beta = \begin{bmatrix} \beta_1 \\ \vdots \\ \beta_{p+m} \end{bmatrix}, \beta_i = \begin{bmatrix} \beta_{i1} \\ \vdots \\ \beta_{ik} \end{bmatrix}$$

$$B = \begin{bmatrix} B_1 & \dots & 0 \\ \vdots & \ddots & \vdots \\ 0 & \dots & B_{p+m} \end{bmatrix} B_i = \begin{bmatrix} \beta_{i1} & \dots & 0 \\ \vdots & \ddots & \vdots \\ 0 & \dots & \beta_{ik} \end{bmatrix}. \quad (16)$$

For group sparsity, the corresponding prior is [8], [17]:

$$p(w_i) = \max_{\gamma_i \geq 0} \mathcal{N}(w_i|0, \gamma_i I) \varphi(\gamma_i)$$

$$p(w) = \prod_{i=1}^{p+m} p(w_i) = \max_{\gamma \geq 0} \mathcal{N}(w|0, \Gamma) \varphi(\gamma) \quad (17)$$

where

$$\gamma = \begin{bmatrix} \gamma_1 \\ \vdots \\ \gamma_{p+m} \end{bmatrix}, \Gamma_i = \begin{bmatrix} \gamma_i & \dots & 0 \\ \vdots & \ddots & \vdots \\ 0 & \dots & \gamma_i \end{bmatrix} \in \mathbb{R}^{k \times k}, \quad (18)$$

$$\Gamma = \begin{bmatrix} \Gamma_1 & \dots & 0 \\ \vdots & \ddots & \vdots \\ 0 & \dots & \Gamma_{p+m} \end{bmatrix}.$$

*Remark 2:* Note that (17) is for a normal group-sparse  $w$ . Considering the dynamical structure function, the last group of  $w$  contains parameters of the denominator of the transfer function and hence cannot be all zero. So in fact, it should be excluded from the group-sparse prior.

To promote both element and group sparsity, we multiply (15) by (17) and normalize it:

$$p(w) = C * \max_{\gamma \geq 0, \beta \geq 0} \mathcal{N}(w|0, B) \mathcal{N}(w|0, \Gamma) \varphi(\beta) \varphi(\gamma) \quad (19)$$

where  $C$  is the normalization constant and can be absorbed by functions  $\varphi(\beta)$  or  $\varphi(\gamma)$ . Hence:

$$p(w) = \max_{\gamma \geq 0, \beta \geq 0} \mathcal{N}(w|0, B) \mathcal{N}(w|0, \Gamma) \varphi(\beta) \varphi(\gamma). \quad (20)$$

We now get a lower bound of the prior as:

$$\begin{aligned} p(w) &\geq \mathcal{N}(w|0, B) \mathcal{N}(w|0, \Gamma) \varphi(\beta) \varphi(\gamma) \\ &= \hat{p}(w). \end{aligned} \quad (21)$$

If either  $\beta_{ij}$  or  $\gamma_i$  is 0, the corresponding Gaussian distribution becomes a Dirac delta function imposing element or group sparsity to  $w$ .

### B. Type II Maximization

Although the implicit prior  $\hat{p}(w)$  is improper, we can still get a normalized posteriori distribution of  $w$  as:

$$\begin{aligned} \hat{p}(w|y) &= \frac{p(y|w) \hat{p}(w)}{\int p(y|w) \hat{p}(w) dw} \\ &= \frac{\mathcal{N}(y|Aw, \Pi) \mathcal{N}(w|0, B) \mathcal{N}(w|0, \Gamma) \varphi(\beta) \varphi(\gamma)}{\int p(y|w) \hat{p}(w) dw}. \end{aligned} \quad (22)$$

Clearly,  $p(w|y)$  is Gaussian since  $\log(p(w|y))$  is a quadratic function of  $w$ :

$$p(w|y) = \mathcal{N}(w|\mu_w, \Sigma_w) \quad (23)$$

where

$$\begin{aligned} \Sigma_w &= [(\Gamma^{-1} + B^{-1}) + A^T \Pi^{-1} A]^{-1} \\ \mu_w &= [(\Gamma^{-1} + B^{-1}) + A^T \Pi^{-1} A]^{-1} A^T \Pi^{-1} y. \end{aligned} \quad (24)$$

Now, the core of the problem is to choose proper hyper-parameters  $\beta$  and  $\gamma$  so that  $\hat{p}(w|y) \approx p(w|y)$  to some extent. One way is to minimize the misaligned mass between  $p(w)$  and  $\hat{p}(w)$  weighted by the marginal likelihood  $p(y|w)$  which is also called evidence maximization or Type II maximization [9], [16], [18]. It is equivalent to estimating all the unknown variables using maximum likelihood method:

$$\begin{aligned} (\gamma, \beta, \Pi) &= \arg \min_{\beta, \gamma \geq 0, \Pi \succeq 0} \int p(y|w) |p(w) - \hat{p}(w)| dw \\ &= \arg \max_{\beta, \gamma \geq 0, \Pi \succeq 0} \int p(y|w) \hat{p}(w) dw \\ &= \arg \min_{\beta, \gamma \geq 0, \Pi \succeq 0} -2 \log \int p(y|w) \hat{p}(w) dw \\ &= \arg \min_{\beta, \gamma \geq 0, \Pi \succeq 0} -2 \log \hat{p}(y|\beta, \gamma, \Pi) \end{aligned} \quad (25)$$

*Remark 3:*  $\Pi$  matrix has a block-diagonal symmetric Toeplitz structure. It is parameterized by  $mk(2M - k + 1)/2$  variables. Estimation of  $\Pi$  is very important because the recovery performance can be poor if estimated  $\Pi$  is sub-optimal [8]. To avoid over-fitting, we assume 1) white Gaussian noise  $e(t)$  in each experiment has same variance (number of variables reduces to  $k(2M - k + 1)/2$ ). 2) Each diagonal block of  $\Pi$  is well approximated by its main diagonal and sub-diagonal elements. Consequently,  $\Pi$  is only parameterized by two variables.

*Proposition 1:* Following (25), the estimation  $w$ , hyper-parameters and noise covariance matrix,  $\Pi$  can be estimated by solving the optimization problem:

$$\begin{aligned} \mathcal{L}(\gamma, \beta, \Pi, w) &= \min_{\beta, \gamma, \Pi, w} (y - Aw)^T \Pi^{-1} (y - Aw) + w^T (\Gamma^{-1} + B^{-1}) w \\ &\quad + \log |B + \Gamma| + \log |\Pi + A(\Gamma^{-1} + B^{-1})^{-1} A^T| \end{aligned} \quad (26)$$

Subject to:

$$\beta \geq 0, \gamma \geq 0, \Pi \succeq 0$$

where we set  $p(\cdot) = -2 \log \varphi(\cdot) = \text{const.}$

*Proof:* The derivation can be found in Section A of Appendix. ■

Now, assume

$$L = (\Gamma^{-1} + B^{-1})^{-1} \quad (27)$$

so that

$$L \leq \Gamma, B = (L^{-1} - \Gamma^{-1}) \quad (28)$$

where

$$L_i = \begin{bmatrix} l_{i1} & \dots & 0 \\ \vdots & \ddots & \vdots \\ 0 & \dots & l_{ik} \end{bmatrix}, L = \begin{bmatrix} L_1 & \dots & 0 \\ \vdots & \ddots & \vdots \\ 0 & \dots & L_p \end{bmatrix} \quad (29)$$

Assuming  $l = \text{diag}(L)$  and substituting (27) into (26) lead to:

$$\begin{aligned} \mathcal{L}(\gamma, l, \Pi, w) &= \min_{\Gamma, L, \Pi, w} (y - Aw)^T \Pi^{-1} (y - Aw) + w^T L^{-1} w \\ &\quad + \log |\Pi + ALA^T| + 2 \log |\Gamma| - \log |\Gamma - L| \end{aligned} \quad (30)$$

subject to:

$$0 \preceq L \preceq \Gamma, \gamma \geq 0, \Pi \succeq 0.$$

### C. Algorithm to solve Type II maximization

Let:

$$\begin{aligned} u(w, \Pi, l, \gamma) &= (y - Aw)^T \Pi^{-1} (y - Aw) + w^T L^{-1} w - \log |\Gamma - L| \\ v(\Pi, l, \gamma) &= -(\log |\Pi + ALA^T| + 2 \log |\Gamma|). \end{aligned} \quad (31)$$

The optimization problem (30) becomes:

$$\mathcal{L}(\gamma, l, \Pi, w) = \min_{\gamma \geq 0, 0 \preceq L \preceq \Gamma, \Pi \succeq 0} u(w, \Pi, l, \gamma) - v(\Pi, l, \gamma). \quad (32)$$

*Proposition 2:* Functions  $u(w, \Pi, l, \gamma)$  and  $v(\Pi, l, \gamma)$  are both jointly convex with respect to their own variables [5].

*Proof:* The derivation can be found in Section B of Appendix. ■

As a result, the cost function actually is a difference of two convex functions and thus is a difference of convex programming (DCP) problem. It can be solved using sequential convex optimization techniques. Here, we use convex-concave procedure (CCCP) which belongs to majorization-minimization (MM) algorithm using the linear majorization

function [4], [24]. For  $\min_x f(x)$  where  $f(x) = u(x) - v(x)$ , and we can solve it iteratively by:

$$x^{n+1} = \arg \min_x u(x) - \langle x, \nabla f(x^n) \rangle \quad (33)$$

where  $\langle \cdot, \cdot \rangle$  denotes inner product.

Therefore, the optimization problem (30) can be decomposed into sequential convex optimization problems:

$$\begin{aligned} & (\gamma^{n+1}, l^{n+1}, \Pi^{n+1}, w^{n+1}) \\ & = \arg \min_{\Gamma, L, \Pi, w} u(w, \Pi, l, \gamma) - \text{tr} [\nabla_{\Pi} v(\Pi^n, l^n, \gamma^n) \Pi] \\ & \quad - \nabla_l^T v(\Pi^n, l^n, \gamma^n) l - \nabla_{\gamma}^T v(\Pi^n, l^n, \gamma^n) \gamma \end{aligned} \quad (34)$$

subject to:

$$0 \leq L \leq \Gamma, \gamma \geq 0, \Pi \succeq 0,$$

where

$$\begin{aligned} -\nabla_{\Pi} v &= (\Pi + ALA^T)^{-1} \\ -\nabla_l v &= \text{diag}\{A^T(\Pi + ALA^T)^{-1}A\} \\ -\nabla_{\gamma} v &= 2k\gamma^{-1}, \gamma^{-1} = \begin{bmatrix} \gamma_1^{-1} \\ \vdots \\ \gamma_p^{-1} \end{bmatrix}. \end{aligned} \quad (35)$$

To alleviate the computation burden at each iteration and generate reasonable estimation of  $\Pi$ , we separate the update of variables in (32) into two steps using Nonlinear Gaussian Seidel method [23].

Step 1:

$$\begin{aligned} \begin{bmatrix} w^{n+1} \\ l^{n+1} \\ \gamma^{n+1} \end{bmatrix} &= \arg \min_{\Gamma \succeq 0, 0 \leq L \leq \Gamma} u(w, \Pi^n, l, \gamma) \\ & \quad - \nabla_l^T v(\Pi^n, l^n, \gamma^n) l - \nabla_{\gamma}^T v(\Pi^n, l^n, \gamma^n) \gamma. \end{aligned} \quad (36)$$

Step 2:

$$\begin{aligned} \Pi^{n+1} &= \arg \min_{\Pi \succeq 0} u(w^{n+1}, \Pi, l^{n+1}, \gamma^{n+1}) \\ & \quad - \text{tr} [\nabla_{\Pi} v(\Pi^n, l^{n+1}, \gamma^{n+1}) \Pi]. \end{aligned} \quad (37)$$

#### D. Solve CCCP by Alternating Direction Method of Multipliers (ADMM)

If the network is large, solving (36) using toolbox like CVX may encounter memory difficulty because the dimension of  $w$  is huge. In this case, we consider to split the optimization problem into a series of independent sub-problems with lower variable dimension. It turns out that the split cost function can be treated as a sharing problem and as a result can be solved using ADMM algorithm [6], [7].

First of all, we partition and rearrange variables in (36):

$$\begin{bmatrix} \frac{w}{l} \\ \gamma \end{bmatrix} \Rightarrow \begin{bmatrix} w_1 \\ l_1 \\ \gamma_1 \\ \vdots \\ w_{p+m} \\ l_{p+m} \\ \gamma_{p+m} \end{bmatrix} \in R^{(p+m)(2k+1) \times 1}, \quad (38)$$

$$\begin{aligned} A &= [A_1 \mid \dots \mid A_{p+m}], \\ A_i &\in R^{Mm \times k}. \end{aligned} \quad (39)$$

Next, we transform (36) into a unconstrained problem by introducing a indicator function:

$$\begin{aligned} \begin{bmatrix} \frac{w}{l} \\ \gamma \end{bmatrix} &= \arg \min_{\Gamma, L} u(w, \Pi, l, \gamma) - \nabla_l^T v(\Pi^n, l^n, \gamma^n) l \\ & \quad - \nabla_{\gamma} v^T(\Pi^n, l^n, \gamma^n) \gamma + \sum_i g(\gamma_i, l_i) \end{aligned} \quad (40)$$

where

$$g(\gamma_i, l_i) = \begin{cases} 0 & \text{if } l_i \geq 0, \gamma_i \geq 0, l_i \leq \gamma_i \\ +\infty & \text{else} \end{cases} \quad (41)$$

Now, we can split the cost function as:

$$\begin{aligned} \begin{bmatrix} w_i \\ l_i \\ \gamma_i \end{bmatrix} &= \arg \min_{\Gamma, L, w} \\ & \left[ \sum_{i=1}^{p+m} w_i^T L_i^{-1} w_i - \log|\Gamma_i - L_i| - \nabla_{l_i}^T l_i - \nabla_{\gamma_i}^T \gamma_i + g(\gamma_i, l_i) \right] \\ & + (y - \sum_{i=1}^{p+m} A_i w_i)^T \Pi^{-1} (y - \sum_{i=1}^{p+m} A_i w_i). \end{aligned} \quad (42)$$

The optimization problem (42) can be then expressed as a sharing problem [6]:

$$\begin{aligned} \begin{bmatrix} w_i \\ l_i \\ \gamma_i \end{bmatrix} &= \arg \min_{\Gamma, L, w} \\ & \left[ \sum_i^{p+m} w_i^T L_i^{-1} w_i - \log|\Gamma_i - L_i| - \nabla_{l_i}^T l_i - \nabla_{\gamma_i} \gamma_i + g(\gamma_i, l_i) \right] \\ & + (y - \sum_{i=1}^{p+m} z_i)^T \Pi^{-1} (y - \sum_{i=1}^{p+m} z_i) \end{aligned}$$

subject to

$$A_i w_i - z_i = 0. \quad (43)$$

Let  $x_i = [w_i^T \ l_i^T \ \gamma_i^T]^T$ , such problem can be solved using scaled ADMM method as [6]:

$$\begin{aligned} x_i^{n+1} &:= \arg \min_{\gamma_i \geq 0, 0 \leq l_i \leq \gamma_i, w_i} w_i^T L_i^{-1} w_i - \log|\Gamma_i - L_i| \\ & \quad - \nabla_{l_i}^T l_i - \nabla_{\gamma_i} \gamma_i + (\rho/2) \|A_i w_i - z_i^n + u_i^n\|_2^2 \\ z^{n+1} &:= \arg \min_z (y - \sum_i z_i)^T \Pi^{-1} (y - \sum_i z_i) \\ & \quad + (\rho/2) \sum_i^n \|z_i - u_i^n - A_i w_i^{n+1}\|_2^2 \\ u_i^{n+1} &:= u_i^n + A_i w_i^{n+1} - z_i^{n+1}. \end{aligned} \quad (44)$$

Clearly, the  $z$ -update still requires to solve a problem in  $Mm(p+m)$  variables. However, we can further simplify the formulation so that the number of variables is reduced to  $Mm$  [6]:

$$\begin{aligned}
x_i^{n+1} &:= \arg \min_{\gamma_i, l_i, w_i} w_i^T L_i^{-1} w_i - \log|\Gamma_i - L_i| - \nabla_{l_i}^T l_i - \nabla_{\gamma_i} \gamma_i \\
&\quad + (\rho/2) \|A_i w_i - A_i w_i^n + \overline{A} w^n - \bar{z}^n + u^n\|_2^2 \\
&\text{subject to:} \\
&\quad \gamma_i \geq 0, 0 \leq l_i \leq \gamma_i \\
\bar{z}^{n+1} &:= \arg \min_{\bar{z}} [y - (p+m)\bar{z}]^T \Pi^{-1} [y - (p+m)\bar{z}] \\
&\quad + [(p+m)\rho/2] \|\bar{z} - u^n - \overline{A} w^{n+1}\|_2^2 \\
u^{n+1} &:= u^n + \overline{A} w^{n+1} - \bar{z}^{n+1},
\end{aligned} \tag{45}$$

where

$$\overline{A} w^n = 1/(p+m) \sum_{i=1}^{p+m} A_i w_i^n. \tag{46}$$

$\bar{z}$ -update can be solved analytically so the algorithm ends with:

$$\begin{aligned}
x_i^{n+1} &:= \arg \min_{\gamma_i, l_i, w_i} w_i^T L_i^{-1} w_i - \log|\Gamma_i - L_i| - \nabla_{l_i}^T l_i - \nabla_{\gamma_i} \gamma_i \\
&\quad + (\rho/2) \|A_i w_i - A_i w_i^n + \overline{A} w^n - \bar{z}^n + u^n\|_2^2 \\
&\text{subject to:} \\
&\quad \gamma_i \geq 0, 0 \leq l_i \leq \gamma_i \\
\bar{z}^{n+1} &:= [2(p+m)I + \rho\Pi]^{-1} (2y + \rho\Pi u^n + \rho\Pi \overline{A} w^{n+1}) \\
u^{n+1} &:= u^n + \overline{A} w^{n+1} - \bar{z}^{n+1}.
\end{aligned} \tag{47}$$

Note that  $x$ -update can be solved in parallel independently.  $\bar{z}$  and  $u$ -update are then solved in sequence after collecting  $x$ -update.

## V. EXTEND TO GENERAL FORMULATION

Inspired by the final optimization problem (30), we can deduce a general formulation of sparsity prior which leads to the same Type-II maximization problem.

Let:

$$p(w) = \max_{\beta \geq 0, \gamma \geq 0} N(w|0, B) \varphi(\beta; \gamma) \varphi(\gamma) \tag{48}$$

so that

$$\hat{p}(w) = N(w|0, B) \varphi(\beta; \gamma) \varphi(\gamma). \tag{49}$$

Following the same Bayesian perspective, we end with the optimization problem:

$$\begin{aligned}
&(\gamma, l, \Pi, w) \\
&= \arg \min_{\Gamma \geq 0, 0 \leq L \leq \Gamma, \Pi \geq 0} (y - Aw)^T \Pi^{-1} (y - Aw) + w^T L^{-1} w \\
&\quad + \log |\Pi + A L A^T| - 2 \log \varphi(l; \gamma) - 2 \log \varphi(\gamma).
\end{aligned} \tag{50}$$

Clearly, if we set  $\varphi(l; \gamma) = |\Gamma - L|^{1/2}$  and  $\varphi(\gamma) = |\Gamma|^{-1}$ , (50) is same with (30).

It is easy to see that prior (48) is still super-Gaussian which means it is a sparsity prior. If we rewrite the lower bound of prior as  $\hat{p}(w) = p(w|L)p(L|\Gamma)P(\Gamma)$  where  $p(L|\Gamma) = \varphi(l; \gamma)$  and  $p(\Gamma) = \varphi(\gamma)$ , the prior actually employs hierarchical Bayesian format. Obviously,  $l$  takes charge of element sparsity of  $w$ .  $p(L|\Gamma)$  brings an underlying constraint  $0 \leq L \leq \Gamma$  which controls sparsity of  $L$ .  $\varphi(\gamma) = |\Gamma|^{-1}$  is similar to a Jeffrey prior inducing element sparsity to  $\gamma$  thus enforcing group sparsity to  $l$  via  $p(L|\Gamma)$ . Therefore, two hyper-parameters in (20) controls element and group sparsity of  $w$  directly while in (48),  $\gamma$  imposes group sparsity to  $w$  indirectly via  $l$ .

The discussion above indicates that it is possible to consider more features of  $w$  at the same time by using hierarchical Bayesian prior. We can assume  $n$  hyper-parameters each of which stands for one feature of  $w$  and impose such feature to the hyper-parameter ranked ahead. Consequently, the prior of  $w$  induces all these features to the estimation.

## VI. SIMULATION

To guarantee the identifiability of the network, we assign a special structure to the matrix  $P$ . We assume there are same number of input as nodes and set  $P$  matrix to be diagonal. Such a network is identifiable following immediately from the Theorem 1 because  $p-1$  elements in each column of  $P$  are known 0. We consider here an LTI system with dynamic structure functions  $Q$  and  $P$  as in eq. (10) with 10 nodes.

We set the maximal order of denominators in  $Q, P$  to  $k=5$ . Time series data from 10 experiment with 30 measurements for each is collected when the input to the system is Gaussian random noise. Since there are 10 measured states and each measured state is controlled by one input, the dictionary matrix has  $(5 \times 11) = 55$  columns and 30 rows. We can correctly identify the topology of  $Q$  by the proposed method.

For comparison purpose, the Type I sparse group lasso [20] is also applied. Figure 1 shows that Type I algorithm has a poor performance, as it picks many incorrect links and misses a correct link. Numerical values of true and identified dynamical structure functions are given in the Supporting Information<sup>1</sup>. The estimated LTI model indicates the performance of the proposed algorithm can be further improved if a proper rule to prune out small elements of  $w$  is adopted.

## VII. CONCLUSION AND DISCUSSION

This paper proposes a method to identify the dynamical structure function assuming its identifiability. The problem is formulated as a linear regression model and solved using sparse Bayesian learning. Given measured time series data from the nodes of the network, the method is able to infer the topology and internal dynamics of the network without any prior knowledge of the system, including its topology or system order. The newly proposed method penalises the complexity of the network by introducing both group

<sup>1</sup>the supporting information of this paper is available from <http://hybrid.eecs.berkeley.edu/~yeyuan/cdc16.pdf>

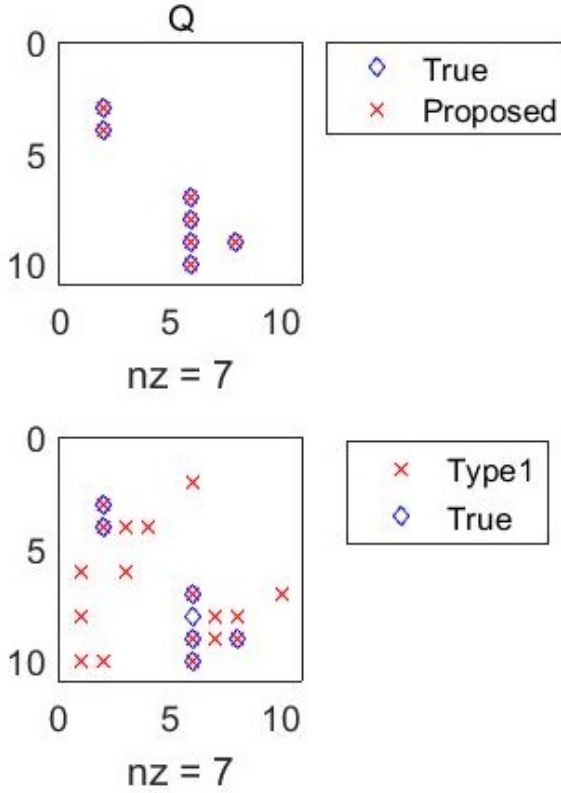

Fig. 1: Topology of  $Q$  matrices. Red x: identified nodes. Blue diamond: True.

and element sparsity. These two kinds of sparse priors are combined and further extended to a general form which reveals their rationality.

To guarantee identifiability, we assumed the data originated from  $p$  (same number as measurements) experiments and that only one input is non-zero for each experiment. However, in reality it may not be feasible to run so many experiments, or having such specific inputs. In that case, the network would probably not be identifiable. Nevertheless, future work will investigate which classes of systems can still reliably be inferred with this method. We expect there will be networks, especially those that are sparse, that can achieve good estimation with a much smaller number of inputs.

## VIII. ACKNOWLEDGEMENT

Duong L.T. Pham and Jorge Goncalves acknowledge the support from the Luxembourgish National Research Fund (FNR 14/BM/8231540). Ye Yuan and Claire J. Tomlin are supported in part by NSF under CPS:ActionWebs (CNS-0931843) and CPS:FORCES (CNS1239166), by NASA under grants NNX12AR18A and UCSCMCA-14-022 (UARC), by ONR under grants N00014-12-1-0609, N000141310341 (Embedded Humans MURI), and MIT\_5710002646 (SMARTS MURI), and by AFOSR under grants UPenn-FA9550-10-1-0567 (CHASE MURI) and the SURE project.

## REFERENCES

- [1] H. Weerts, A. Dankers, P. Hof Identifiability in dynamic network identification, *IFAC-PapersOnLine*, 48(28), 2015, pp. 1409-1414.
- [2] B. Sanandaji, T. Vincent, M. Wakin A review of sufficient conditions for structure identification in interconnected systems, *Proceedings of the 16th IFAC Symposium on System Identification*, 2012, pp. 1623-1628.
- [3] N. Everitt, G. Bottegal, C. Rojas, H. Hjalmarsson On the Effect of Noise Correlation in Parameter Identification of SIMO Systems, *IFAC-PapersOnLine*, vol. 48(28), 2015, pp. 326-331.
- [4] T. Chen, M.S. Andersen, L. Ljung, A. Chiuso, and G. Pillonetto, System identification via sparse multiple kernel-based regularization using sequential convex optimization techniques, *IEEE Trans. Automat. Contr.*, vol. 59(11), 2014, pp. 2933-2945.
- [5] S. Boyd, and L. Vandenberghe *Convex Optimization*, Cambridge University Press; 2004.
- [6] S. Boyd, Distributed Optimization and Statistical Learning via the Alternating Direction Method of Multipliers, *Found. Trends Mach. Learn.*, vol. 3(1), 2010, pp. 1-122.
- [7] W. Pan, A. Sootla, and G. B. Stan, Distributed reconstruction of nonlinear networks: An ADMM approach, *IFAC Proc. Vol.*, vol. 19, 2014, pp. 3208-3213.
- [8] Z. Zhang and B. D. Rao, Extension of SBL algorithms for the recovery of block sparse signals with intra-block correlation, *IEEE Trans. Signal Process.*, vol. 61(8), 2013, pp. 2009-2015.
- [9] C. Bishop. *Pattern recognition and machine learning*, Springer New York; 2006.
- [10] D. J. Wilkinson. *Stochastic Modelling for Systems Biology*, CRC Press; 2012.
- [11] J. Goncalves and S. Warnick Necessary and sufficient conditions for dynamical structure reconstruction of LTI networks, *IEEE Trans. Automat. Contr.*, vol. 53(7), 2008, pp. 1670-1674.
- [12] Y. Yuan, G. Stan, S. Warnick, and J. Goncalves, Robust dynamical network structure reconstruction, *Automatica*, vol. 47, 2011, pp. 1230-1235.
- [13] P. M. J. Van den Hof, A. Dankers, P. S. C. Heuberger and X. Bombois, Identification of dynamic models in complex networks with prediction error methods - basic methods for consistent module estimates, *Automatica*, vol. 49, no. 10, 2013, pp. 2994-3006.
- [14] A. Dankers, P. M. J. Van den Hof, P. S. C. Heuberger and X. Bombois, Dynamic network identification using the direct prediction-error method, *Proceedings of 51st IEEE Conference on Decision and Control*, 2012.
- [15] D. Materassi and M. V. Salapaka, On the problem of reconstructing an unknown topology via locality properties of the wiener filter, *IEEE Trans. Automat. Contr.*, vol. 57(7), 2012, pp. 1765-1777.
- [16] W. Pan, Y. Yuan, J. Goncalves, and G. Stan A Sparse Bayesian Approach to the Identification of Nonlinear State-Space Systems, *IEEE Trans. Automat. Contr.*, vol. 61(1), 2016, pp. 182-187.
- [17] W. Pan, Y. Yuan, L. Ljung, J. Goncalves, and G. Stan Identifying biochemical reaction networks using heterogeneous datasets, *CDC*, 2015.
- [18] D. P. Wipf, B. D. Rao, and S. Nagarajan Latent Variable Bayesian Models for Promoting Sparsity, *IEEE Trans. Inf. Theory.*, vol. 57(9), 2011, pp. 6236-6255.
- [19] S. Babacan, S. Nakajima, and M. Do Bayesian group-sparse modeling and variational inference, *Signal Process. IEEE Trans.*, vol. 62(11), 2014, pp. 2906-2921.
- [20] N. Simon, J. Friedman, T. Hastie, and R. Tibshirani A Sparse-Group Lasso, *J. Comput. Graph. Stat.*, vol. 22(2), 2013, pp. 231-245.
- [21] K. Lee and R. Chen BSGS: Bayesian Sparse Group Selection, *The R Journal.*, vol. 7(2), 2015, pp. 122-133.
- [22] M. Tipping Sparse Bayesian Learning and the Relevance Vector Mach, *J. Mach. Learn. Res.*, vol. 1, 2001, pp. 211-244.
- [23] C. Nazonale and D. Ricerche On the convergence of the block nonlinear Gauss-Seidel method under convex constraints, 1998
- [24] B. K. Sriperumbudur On the Convergence of the Concave-Convex Procedure, *Nips.*, vol. 1, 2009, pp. 1-9.
- [25] J. Palmer, D. Wipf, K. Kreutz-Delgado, and B. Rao Variational EM algorithms for non-Gaussian latent variable models, *Adv. Neural Inf. Process. Syst.*, vol. 18, 2006, pp. 1059.

## APPENDIX

### A. Derivation of Type II maximization problem

Firstly, note that:

$$\begin{aligned}
& -2 \log \int p(y|w) \hat{p}(w) dw \\
& -2 \log \int \mathcal{N}(y|Aw, \Pi) \mathcal{N}(w|0, B) \mathcal{N}(w|0, \Gamma) \varphi(\beta) \varphi(\gamma) dw \\
& -2 \log \int \exp(E_w) dw + \log |\Pi| + \log |B| + \log |\Gamma| dw
\end{aligned} \tag{51}$$

where

$$E_w = -\frac{1}{2}[(y - Aw)^T \Pi^{-1} (y - Aw) + (w^T (B^{-1} + \Gamma^{-1}) w)] \tag{52}$$

ignoring all the constant terms.

By completing the square:

$$\begin{aligned}
& -\frac{1}{2}(y - Aw)^T \Pi^{-1} (y - Aw) - \frac{1}{2}w^T (\Gamma^{-1} + B^{-1}) w \\
& = -\frac{1}{2}[(w - \mu_w)^T \Sigma_w^{-1} (w - \mu_w) + E_y]
\end{aligned} \tag{53}$$

where

$$\begin{aligned}
\Sigma_w &= [(\Gamma^{-1} + B^{-1}) + A^T \Pi^{-1} A]^{-1} \\
\mu_w &= [(\Gamma^{-1} + B^{-1}) + A^T \Pi^{-1} A]^{-1} A^T \Pi^{-1} y \\
E_y &= \min_w (y - Aw)^T \Pi^{-1} (y - Aw) + w^T (\Gamma^{-1} + B^{-1}) w
\end{aligned} \tag{54}$$

In addition, note that:

$$\begin{aligned}
& -2 \log \int \exp \left\{ -\frac{1}{2}[(w - \mu_w)^T \Sigma_w^{-1} (w - \mu_w)] \right\} dw \\
& = -\log |\Sigma_w| \\
& = \log |(\Gamma^{-1} + B^{-1}) + A^T \Pi^{-1} A|
\end{aligned} \tag{55}$$

ignoring all the constant terms.

Using (53) and (55), the integral in (51) becomes:

$$\begin{aligned}
& -2 \log \int p(y|w) \hat{p}(w) dw \\
& = E_y + \log |(\Gamma^{-1} + B^{-1}) + A^T \Pi^{-1} A| \\
& + \log |\Pi| + \log |B| + \log |\Gamma| \\
& = E_y + \log |(\Gamma^{-1} + B^{-1}) + A^T \Pi^{-1} A| - \log |(\Gamma^{-1} + B^{-1})| \\
& + \log |(\Gamma^{-1} + B^{-1})| + \log |\Pi| + \log |B| + \log |\Gamma| \\
& = E_y + \log |I + (\Gamma^{-1} + B^{-1})^{-1} A^T \Pi^{-1} A| \\
& + \log |(\Gamma + B)| + \log |\Pi| \\
& = E_y + \log |I + \Pi^{-1} A (\Gamma^{-1} + B^{-1})^{-1} A^T| \\
& + \log |(\Gamma + B)| + \log |\Pi| \\
& = E_y + \log |\Pi + A (\Gamma^{-1} + B^{-1})^{-1} A^T| + \log |(\Gamma + B)| \\
& = \min_w (y - Aw)^T \Pi^{-1} (y - Aw) + w^T (\Gamma^{-1} + B^{-1}) w \\
& + \log |\Pi + A (\Gamma^{-1} + B^{-1})^{-1} A^T| + \log |(\Gamma + B)|.
\end{aligned} \tag{56}$$

Inserting (56) back to (25), we get:

$$\begin{aligned}
& \mathcal{L}(\gamma, \beta, \Pi, w) \\
& = \min_{\beta, \gamma, \Pi, w} (y - Aw)^T \Pi^{-1} (y - Aw) + w^T (\Gamma^{-1} + B^{-1}) w \\
& + \log |B + \Gamma| + \log |\Pi + A (\Gamma^{-1} + B^{-1})^{-1} A^T|
\end{aligned}$$

Subject to:

$$\beta \geq 0, \gamma \geq 0, \Pi \succeq 0. \tag{57}$$

### B. Convexity of DCP problem

To see functions  $u(w, \Pi, l, \gamma)$  and  $v(\Pi, l, \gamma)$  are jointly convex functions, we need to prove each term is jointly convex.

For  $u(w, \Pi, l, \gamma)$ , we see that

$$\begin{aligned}
& \Pi \succ 0, \quad (y - Aw)^T \Pi^{-1} (y - Aw) < t \\
& \text{equivalent to} \\
& \begin{bmatrix} \Pi & y - Aw \\ (y - Aw)^T & t \end{bmatrix} \succ 0
\end{aligned} \tag{58}$$

so the term  $(y - Aw)^T \Pi^{-1} (y - Aw)$  is jointly convex as is same with  $w^T L^{-1} w$ .

For the term  $-\log |\Gamma - L|$ , firstly  $-\log |\cdot|$  is a convex function in  $S^+$ . Since  $\Gamma - L$  is an affine function of  $\Gamma$  and  $L$ ,  $-\log |\Gamma - L|$  is jointly convex. The convexity of function  $v(\Pi, l, \gamma)$  can be seen in the same way as function  $-\log |\Gamma - L|$ .

## Supporting Information

### C. Dynamical structure function

True dynamical structure functions that were used for data generation

$$\begin{aligned}
 y_1(t) &= \frac{0.1427 + 0.275z^{-1} + 0.42z^{-2}}{1 + 0.4z^{-1} - 0.27z^{-2} + 0.04z^{-3}}u_1(t) + \frac{1 + 0.01z^{-1}}{1 + 0.4z^{-1} - 0.27z^{-2} + 0.04z^{-3}}e_1(t) \\
 y_2(t) &= \frac{-0.0153 + 0.3862z^{-1}}{1 + 0.5z^{-1} + 0.06z^{-2}}u_2(t) + \frac{1 + 0.01z^{-1} + 0.02z^{-2}}{1 + 0.5z^{-1} - 0.06z^{-2}}e_2(t) \\
 y_3(t) &= \frac{-0.3z^{-1} - 0.5z^{-2}}{1 + 1.55z^{-1} + 0.8z^{-2} + 0.15z^{-3}}y_2 + \frac{0.831 - 0.707z^{-1} + 0.61z^{-2}}{1 + 1.55z^{-1} + 0.8z^{-2} + 0.15z^{-3}}u_3(t) + \frac{1}{1 + 1.55z^{-1} + 0.8z^{-2} + 0.15z^{-3}}e_3(t) \\
 y_4(t) &= \frac{-0.2z^{-1} - 0.1z^{-2}}{1 - 0.7z^{-1} + 0.1z^{-2}}y_2 + \frac{0.8195 - 0.68z^{-1} + 0.59z^{-2}}{1 - 0.7z^{-1} + 0.1z^{-2}}u_4(t) + \frac{1 + 0.89z^{-1}}{1 - 0.7z^{-1} + 0.1z^{-2}}e_4(t) \\
 y_5(t) &= \frac{-1.502 + 1.627z^{-1}}{1 + 1.4z^{-1} + 0.98z^{-2}}u_5(t) + \frac{1 + 0.075z^{-1}}{1 + 1.4z^{-1} + 0.98z^{-2}}e_5(t) \\
 y_6(t) &= \frac{1.214}{1 + 0.35z^{-1}}u_6(t) + \frac{1 + 0.02z^{-1}}{1 + 0.35z^{-1}}e_6(t) \\
 y_7(t) &= \frac{-0.35}{1 + 0.55z^{-1}}y_6(t) + \frac{-0.7642}{1 + 0.55z^{-1}}u_7(t) + \frac{1 + 0.03z^{-1}}{1 + 0.55z^{-1}}e_7(t) \\
 y_8(t) &= \frac{-0.55}{1 + 0.49z^{-1}}y_6(t) + \frac{0.038}{1 + 0.49z^{-1}}u_8(t) + \frac{1 + 0.049z^{-1}}{1 + 0.49z^{-1}}e_8(t) \\
 y_9(t) &= \frac{-0.35}{1 + 0.6z^{-1}}y_6(t) + \frac{-0.49}{1 + 0.6z^{-1}}y_8(t) + \frac{0.9347}{1 + 0.6z^{-1}}u_9(t) + \frac{1 + 0.01z^{-1}}{1 + 0.6z^{-1}}e_9(t) \\
 y_{10}(t) &= \frac{-0.25}{1 + 0.8z^{-1}}y_6(t) + \frac{0.8}{1 + 0.8z^{-1}}u_{10}(t) + \frac{1 + 0.04z^{-1}}{1 + 0.8z^{-1}}e_{10}(t)
 \end{aligned}$$

The identified dynamic structure functions by the proposed method are

$$\begin{aligned}
 y_1(t) &= \frac{0.15 + 0.28z^{-1} + 0.402z^{-2}}{1 + 0.366z^{-1} - 0.26z^{-2} + 0.035z^{-3}}u_1(t) \\
 y_2(t) &= \frac{-0.02 - 0.3805z^{-1}}{1 + 0.469z^{-1} - 0.05383z^{-2}}u_2(t) \\
 y_3(t) &= \frac{-0.3005z^{-1} - 0.48z^{-2}}{1 + 1.56z^{-1} + 0.7913z^{-2} + 0.105z^{-3}}y_2 + \frac{0.8195 - 0.68z^{-1} + 0.59z^{-2}}{1 + 1.56z^{-1} + 0.7913z^{-2} + 0.105z^{-3}}u_3(t) \\
 y_4(t) &= \frac{-0.1909z^{-1} - 0.67z^{-2}}{1 - 0.751z^{-1} + 0.1089z^{-2}}y_2 + \frac{0.8195 - 0.68z^{-1} + 0.59z^{-2}}{1 - 0.751z^{-1} + 0.1089z^{-2}}u_4(t) \\
 y_5(t) &= \frac{-1.532 + 1.67z^{-1}}{1 + 1.4z^{-1} + 0.98z^{-2}}u_5(t) \\
 y_6(t) &= \frac{1.19}{1 + 0.36z^{-1}}u_6(t) \\
 y_7(t) &= \frac{-0.2958}{1 + 0.54z^{-1}}y_6(t) + \frac{-0.7625}{1 + 0.54z^{-1}}u_7(t) \\
 y_8(t) &= \frac{-0.55}{1 + 0.475z^{-1} + 0.026z^{-2}}y_6(t) + \frac{0.0341}{1 + 0.475z^{-1} + 0.026z^{-2}}u_8(t)
 \end{aligned}$$

$$y_9(t) = \frac{-0.3413}{1 + 0.602z^{-1}}y_6(t) + \frac{-0.4829 + 0.0085z^{-1}}{1 + 0.602z^{-1}}y_8(t) + \frac{0.9147}{1 + 0.602z^{-1}}u_9(t)$$

$$y_{10}(t) = \frac{-0.21}{1 + 0.73z^{-1}}y_6(t) + \frac{0.76 + 0.04z^{-1}}{1 + 0.73z^{-1}}u_{10}(t)$$

From the identified dynamic structure functions, it can be seen that the causal relationships between  $(y_3, y_2)$ ;  $(y_4, y_2)$ ;  $(y_7, y_6)$ ;  $(y_8, y_6)$ ;  $(y_9, y_8, y_6)$  are almost correctly identified.
